# Supplementary material for: Boosting Studies of Multi-Agent Reinforcement Learning on Google Research Football Environment: the Past, Present, and Future
Source: arXiv:2309.12951 source file (2023-09-22)
Supplement: Supplementary file 1 [file appendixD.tex]

\section{Algorithms}\label{appendix: algos}

%\jh{we may don't need this appendix}

In this section, we discuss the benchmark algorithm we adopt for our experiments.

\subsection{QMIX and QPLEX}

\subsection{Independent PPO (IPPO) and Multi-agent PPO (MAPPO)}

\subsection{HAPPO and A2PO}

\subsection{Multi-agent Transformer}
